# Supplementary material for: Learning to Construct 3D Building Wireframes from 3D Line Clouds
Source: arXiv:2208.11948 source file (2022-11-04)
Supplement: Supplementary file 1 [file tb_suppl_runtime.tex]

\centering
\scriptsize
{\tabcolsep=0.65em
\begin{tabular}{lcccccccc}
\toprule[0.8pt]
\multicolumn{1}{c}{Method} & \begin{tabular}[c]{@{}c@{}}Data prep.\end{tabular} & \begin{tabular}[c]{@{}c@{}}pre-processing\end{tabular} & \begin{tabular}[c]{@{}c@{}}junc. pred.\end{tabular} & \begin{tabular}[c]{@{}c@{}}edge pred.\end{tabular} & \begin{tabular}[c]{@{}c@{}}plane pred.\end{tabular} & \begin{tabular}[c]{@{}c@{}}surf. recon.\end{tabular} & \begin{tabular}[c]{@{}c@{}}post-processing\end{tabular} & Total \\ \midrule[0.8pt]
line3Dpp & 19.5 & \cellcolor{babyblue!15}13.9 & - & \cellcolor{babyblue!15}- & - & \cellcolor{babyblue!15}- & - & \cellcolor{babyblue!15}33.1 \\
line2Surf & 33.1 & \cellcolor{babyblue!15}- & - & \cellcolor{babyblue!15}- & 163.2 & \cellcolor{babyblue!15}57.6 & 0.21 & \cellcolor{babyblue!15}253.9 \\
PolyFit & 63.8 & \cellcolor{babyblue!15}- & - & \cellcolor{babyblue!15}- & 40.4 & \cellcolor{babyblue!15}5.64 & 0.067 & \cellcolor{babyblue!15}110.0 \\
PC2WF & 63.8 & \cellcolor{babyblue!15}5.21 & 4.94 & \cellcolor{babyblue!15}26.1 & - & \cellcolor{babyblue!15}- & 0.15 & \cellcolor{babyblue!15}100.2 \\ \midrule[0.5pt]
Ours & 19.5 & \cellcolor{babyblue!15}- & 0.18 & \cellcolor{babyblue!15}0.72 & - & \cellcolor{babyblue!15}- & 0.012 & \cellcolor{babyblue!15}20.4 \\ \bottomrule[0.8pt]
\end{tabular}
}
